# Supplementary material for: Ousiometrics: The essence of meaning aligns with a power-danger-structure framework instead of valence-arousal-dominance
Source: arXiv:2110.06847 ancillary file (2026-06-03)

~ danger-structure ousiogram for the NRC VAD lexicon ~

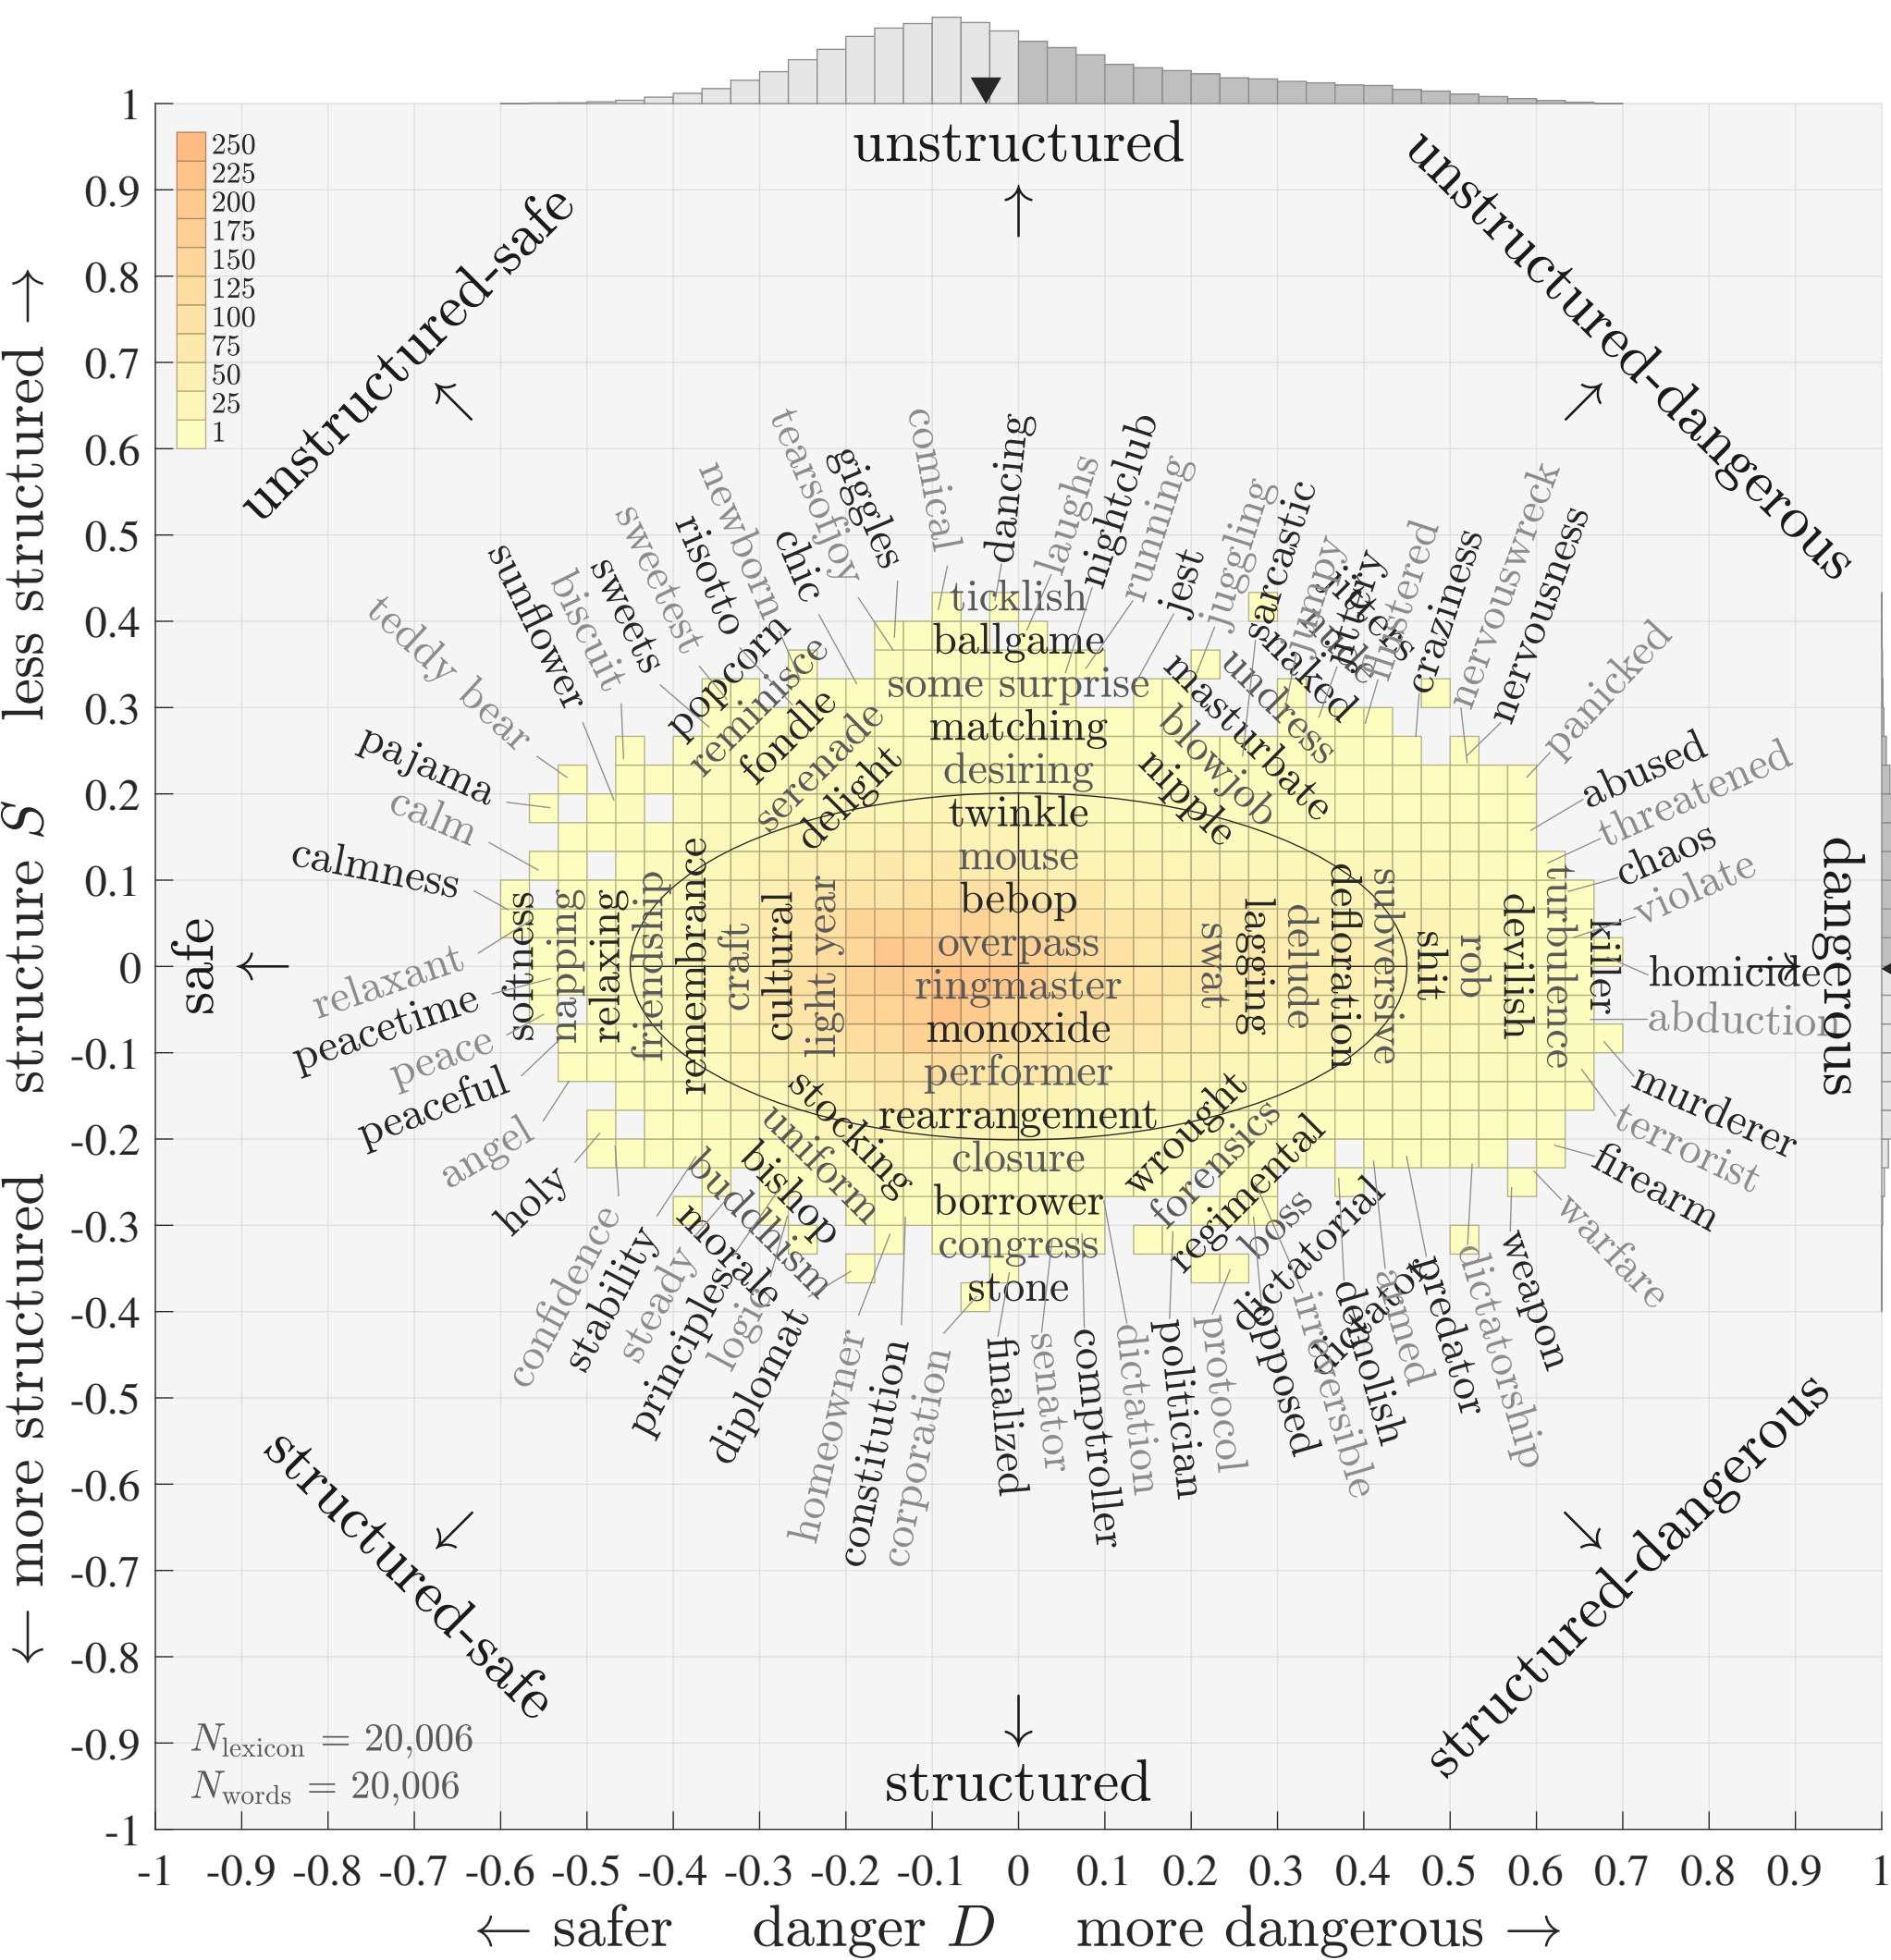

Supplement: Supplementary file 1 [file ousiograms_VAD_GES_PDS_allpairs.pdf]
